# Supplementary material for: Detecting Bad Smells in Use Case Descriptions
Source: arXiv:2009.01542 source file (2020-09-03)
Supplement: Supplementary file 1 [file appendix.pdf]

# Appendix of "Detecting Bad Smells in Use Case Descriptions"

Yotaro Seki, Shinpei Hayashi, and Motoshi Saeki
School of Computing, Tokyo Institute of Technology
Ookayama 2–12–1, Meguro-ku, Tokyo 152–8550, Japan
Email: {yotaro,hayashi,saeki}@se.cs.titech.ac.jp

***Abstract*—This article is an appendix of our paper entitled "Detecting Bad Smells in Use Case Descriptions" to be published in proceedings of the 27th IEEE International Requirements Engineering Conference (RE'19) [1].**

## I. Selected Use Case Descriptions for Inspection

Table I shows the list of used use case descriptions that have been selected for the inspection of bad smells in them. In the table, the columns indicate the ID (ID), the name of the target use case (Name), the domain of the use case (Domain), the description when available (Description), the source information (Source), the numbers of basic steps ($B$), exception steps ($E$), and alternate steps ($A$). The descriptions U01–30 were used for the analysis in Section II in the original paper [1]. The descriptions U30–38 were used for the controlled experiment in Section III in the original paper [1]. Since the original name and description are in Japanese, we translated them into English. The domain information was not extracted from the sources but was derived by the authors. For the items that we retrieved the source information via a web search, the symbols explaining the way how they were searched are attached. We used both Google Search (ⓢ) and Google Image Search (ⓘ), and two different queries (ⓤ and ⓦ).

## II. Comparison among Catalogues

Table II shows our comparison result of smell catalogues. In the table, rows indicate smells defined in our paper, and columns indicate the smells defined in existing three catalogues: Phalp *et al.* [5], Törner *et al.* [6], and Anda and Sjøberg [7]. If a smell defined by us matches with a smell defined in other catalogues, the symbol ✓ is filled in the associated cell.

We show the smells defined in other three catalogues as follows.

*P: Phalp et al. [5]:*

**P01:** Coverage: Scope
**P02:** Coverage: Span
**P03:** Cogent: Text Order
**P04:** Cogent: Dependencies
**P05:** Cogent: Rational Answer
**P06:** Coherent
**P07:** Consistent Abstraction
**P08:** Consistent Structure: Variations
**P09:** Consistent Structure: Sequence
**P10:** Consistent Grammar
**P11:** Consideration of Alternatives: Separation
**P12:** Consideration of Alternatives: Viable
**P13:** Consideration of Alternatives: Numbering

*T: Törner et al. [6]:*

**T01:** Completeness: Missing element (C1)
**T02:** Completeness: Goal not achieved (C2)
**T03:** Correctness: Incorrect flow (C3)
**T04:** Correctness: Outside scope (C4)
**T05:** Consistency: Inconsistent step numbering (C5)
**T06:** Consistency: Irrelevant steps (C6)
**T07:** Consistency: Use Case Decomposition (C7)
**T08:** Readability: Misuse of alternative flows (C8)
**T09:** Unambiguity: Unclear alternative flow condition (C9)
**T10:** Unambiguity: Incorrect linguistics (C10)
**T11:** Level of detail (C11)
**T12:** Misuse of preconditions (C12)

*A: Anda and Sjøberg [7]:*

**A01:** ⟨*Omissions*, *Actors*⟩: Human users or external entities that will interact with the system are not identified
**A02:** ⟨*Omissions*, *Use cases*⟩: Required functionality is not described in use cases. Actors have goals that do not have corresponding use cases
**A03:** ⟨*Omissions*, *Flow of events*⟩: Input or output for use cases is not described. Events that are necessary for understanding the use cases are missing
**A04:** ⟨*Omissions*, *Variations*⟩: Variations that may occur when attempting to achieve the goal of a use case are not specified
**A05:** ⟨*Omissions*, *Relation between use cases*⟩: Common functionality is not separated out in included use cases
**A06:** ⟨*Omissions*, *Trigger, pre- and post-conditions*⟩: Trigger, pre- or post-conditions have been omitted
**A07:** ⟨*Incorrect facts*, *Actors*⟩: Incorrect description of actors or wrong connection between actor and use case
**A08:** ⟨*Incorrect facts*, *Use cases*⟩: Incorrect description of a use case
**A09:** ⟨*Incorrect facts*, *Flow of events*⟩: Incorrect description of one or several events

**A10:** ⟨*Incorrect facts*, *Variations*⟩: Incorrect description of a variation

**A11:** ⟨*Incorrect facts*, *Trigger, pre- and post-conditions*⟩: Incorrect assumptions or results have led to incorrect pre- or post-conditions

**A12:** ⟨*Inconsistencies*, *Actors*⟩: Description of actor is inconsistent with its behavior in use cases

**A13:** ⟨*Inconsistencies*, *Use cases*⟩: Description is inconsistent with reaching the goal of the use case

**A14:** ⟨*Inconsistencies*, *Flow of events*⟩: Events that are inconsistent with reaching the goal of the use case they are part of

**A15:** ⟨*Inconsistencies*, *Variations*⟩: Variations that are inconsistent with the goal of the use case

**A16:** ⟨*Inconsistencies*, *Relation between use cases*⟩: Inconsistencies between diagram and descriptions, inconsistent terminology, inconsistencies between use cases, or different level of granularity

**A17:** ⟨*Inconsistencies*, *Trigger, pre- and post-conditions*⟩: Pre- or post-conditions are inconsistent with goal or flow of events

**A18:** ⟨*Ambiguities*, *Actors*⟩: Too broadly defined actors or ambiguous description of actor

**A19:** ⟨*Ambiguities*, *Use cases*⟩: Name of use case does not reflect the goal of the use case

**A20:** ⟨*Ambiguities*, *Flow of events*⟩: Ambiguous description of events, perhaps because of too little detail

**A21:** ⟨*Ambiguities*, *Variations*⟩: Ambiguous description of what leads to a particular variation

**A22:** ⟨*Ambiguities*, *Trigger, pre- and post-conditions*⟩: Ambiguous description of trigger, pre- or post-condition

**A23:** ⟨*Extraneous information*, *Actors*⟩: Actors that do not derive value from/provide value to the system

**A24:** ⟨*Extraneous information*, *Use cases*⟩: Use cases with functionality outside the scope of the system or use cases that duplicate functionality

**A25:** ⟨*Extraneous information*, *Flow of events*⟩: Superfluous steps or too much detail in steps

**A26:** ⟨*Extraneous information*, *Variations*⟩: Variations that are outside the scope of the system

**A27:** ⟨*Extraneous information*, *Trigger, pre- and post-conditions*⟩: Superfluous trigger, pre- or post-conditions

## III. Definition of Use Case Description Smells

All the definitions of bad smells in use case descriptions defined in our paper are as follows.

---

**Name:** Unordered Flow
**Characteristic:** *Ambiguity*
**Scope:** *Section*
**Symptom:** Some flows are not ordered correctly, and they lead to the difficulties in understanding the behavior of the use case.
**How to Detect:**

- The ID number (briefly ID) of a basic flow starts with 1? (*BasicFlowStartWith1?*)
- The ID of an alternate flow starts with 1? (*AltetrnateFlowStartWith1?*)
- The ID of an exception flow starts with 1? (*ExceptionFlowStartWith1?*)
- Each flow of a basic flow is numbered? (*BasicFlowNumberd?*)
- Each flow of an alternate flow is numbered? (*AlternateFlowNumbered?*)
- Each flow of an exception flow is numbered? (*ExceptionFlowNumbered?*)
- The numbering of a basic flow is incremented by 1? (*BasicFlowOrdered?*)
- The numbering of an alternate flow is incremented by 1? (*AlternateFlowOrdered?*)
- The numbering of an exception flow is incremented by 1? (*ExceptionFlowOrdered?*)

---

**Name:** Origin-Free Exception Flow
**Characteristic:** *Ambiguity*
**Scope:** *Section*
**Symptom:** The origin of an exception flow, i.e., the source of branching to the exception flow, is not specified. It leads to making it difficult to follow the overall flow of the use case.
**How to Detect:** It is described in the exception flow at which sentences the exception for branching to the exception flow may occur in the basic flow? (*ExceptionFlowsOriginDescribed?*)

---

**Name:** Origin-Free Alternate Flow
**Characteristic:** *Ambiguity*
**Scope:** *Section*
**Symptom:** The origin of an alternate flow, i.e., the source of branching to the alternate flow, is not specified. It leads to making it difficult to follow the overall flow of the use case.
**How to Detect:** It is described in the alternate flow at which sentences in the basic flow the alternate flow may start to be executed? (*AlternateFlowsOriginDescribed?*)

---

**Name:** Unclear Feasibility
**Characteristic:** *Sentence*
**Scope:** *Ambiguity*
**Symptom:** An action denoted by a sentence may be required to satisfy conditions before its execution, but these conditions cannot be certified to hold. For example, an action requires some input data for its execution, but their existence cannot be certified at the point of the sentence. It is necessary to walk through the flow that includes the sentence.
**How to Detect:** –

---

**Name:** Origin-Free Operation Result

**Characteristic:** *Ambiguity*
**Scope:** *Sentence*
**Symptom:** The sentence includes the description of the result of execution before, but it is not specified where the described result is obtained. It is time-consuming to explore the reference to the execution point where the result is generated.
**How to Detect:** –

---

**Name:** Sentence Interpretable as Multiple Meaning
**Characteristic:** *Ambiguity*
**Scope:** *Sentence*
**Symptom:** An action denoted by a sentence cannot be uniquely decided. It depends on readers of the sentence, and they may not be able to understand the sentence correctly.
**How to Detect:** –

---

**Name:** Pronoun
**Characteristic:** *Ambiguity*
**Scope:** *Word*
**Symptom:** The occurrence of a pronoun may provide ambiguity on what it denotes.
**How to Detect:** There is an occurrence of pronouns? (NOP > 0)

---

**Name:** Omitted Word
**Characteristic:** *Ambiguity*
**Scope:** *Word*
**Symptom:** Omitting a word may lead to the lack of the necessary information in a sentence, and it can be ambiguous.
**How to Detect:** –

---

**Name:** "Actor" Actor
**Characteristic:** *Ambiguity*
**Scope:** *Word*
**Symptom:** The subject of a sentence denoting an action is "Actor" and a concrete object who performs the action may not be uniquely decided, i.e., ambiguous.
**How to Detect:** There is an occurrence of the word "Actor" in a sentence? (NON("Actor") > 0)

---

**Name:** Unexplained Main Actor
**Characteristic:** *Ambiguity*
**Scope:** *Word*
**Symptom:** The word that is not "System" or that is not specified in Actor section is used as a subject of a sentence denoting an action. It is time-consuming to understand who is essentially an actor.
**How to Detect:** –

---

**Name:** Different Concepts by Same Word
**Characteristic:** *Ambiguity*
**Scope:** *Word*
**Symptom:** A word is used to represent different concepts. The meaning of the word is ambiguous.
**How to Detect:** –

---

**Name:** Omitted Attribute
**Characteristic:** *Ambiguity*
**Scope:** *Word*
**Symptom:** The operation to an object is represented in a sentence, but the operation is actually not to the object but its attribute. An object is confused with its attribute. It may cause misunderstanding of the meaning of the operation.
**How to Detect:** –

---

**Name:** Flow Does Not Meet Precondition
**Characteristic:** *Incorrectness*
**Scope:** *Section*
**Symptom:** A flow does not satisfy a precondition at starting its execution. In this case, the flow cannot be correctly executed.
**How to Detect:** –

---

**Name:** Postcondition Not Satisfied
**Characteristic:** *Incorrectness*
**Scope:** *Section*
**Symptom:** At the termination of the flow, a postcondition is not satisfied. In this case, the flow cannot be correctly executed.
**How to Detect:** –

---

**Name:** Name Does Not Explain Content
**Characteristic:** *Incorrectness*
**Scope:** *Section*
**Symptom:** The name of a use case does not represent its essential content. It causes its misunderstanding.
**How to Detect:** –

---

**Name:** Under or Over Condition
**Characteristic:** *Incorrectness*
**Scope:** *Section*
**Symptom:** Preconditions and/or postconditions include redundant conditions, or some of them are missing. In the case of redundant conditions, additional actions may be required to satisfy the redundant conditions. On the other hand, in the case of missing conditions, an action to satisfy the missing condition may also be missing. In both cases, the flow cannot be correct to the real execution and cannot satisfy the requirements.
**How to Detect:** –

---

**Name:** Much or Less Actors
**Characteristic:** *Incorrectness*
**Scope:** *Section*

**Symptom:** There is an actor in a flow, but it does not appear in the Actor section. On the other hand, there is an actor appearing in the Actor section, but it does not occur in the flow sections. In the former case, there are two possibilities: 1) an action performed by the actor is missing, or 2) the actor is redundant. In the latter case, it causes misunderstanding of the actor because of lacking information of the actor.
**How to Detect:** –

---

**Name:** Contradicted Sentences
**Characteristic:** *Incorrectness*
**Scope:** *Sentence*
**Symptom:** More than one sentence is contradicted to each other. Either of them may be incorrect.
**How to Detect:** –

---

**Name:** Behavior Ignores Condition
**Characteristic:** *Incorrectness*
**Scope:** *Sentence*
**Symptom:** An action denoted by a sentence is executed without satisfying its conditions that should hold before executing it. In this case, another action that should be executed before may be lacking, or the conditions may be wrong.
**How to Detect:** –

---

**Name:** Multiple Situations
**Characteristic:** *Granularity*
**Scope:** *Usecase*
**Symptom:** In a use case description of a use case, multiple different situations are assumed. The use case description is not decomposed at a sufficient level, and it should be decomposed into several use cases.
**How to Detect:** –

---

**Name:** Multiple Exception Flows at an Exception Branch Condition
**Characteristic:** *Granularity*
**Scope:** *Section*
**Symptom:** There are multiple exception flows which start with the same condition. It may cause a misunderstanding that different exceptions exist. It should be merged to a single exception flow.
**How to Detect:** Are there multiple occurrences of branches at the alphabetically same exception condition? (NOEFR > 1)

---

**Name:** Multiple Alternate Flows at an Alternate Branch Condition
**Characteristic:** *Granularity*
**Scope:** *Section*
**Symptom:** There are multiple alternate flows which start with the same condition. It may cause a misunderstanding that different alternatives exist. It should be merged into a single alternate flow.
**How to Detect:** Are there multiple occurrences of branches at the alphabetically same alternate condition? (NOAFR > 0)

---

**Name:** Multiple Roles of an Actor
**Characteristic:** *Granularity*
**Scope:** *Section*
**Symptom:** The different roles are assigned to a word denoting an actor. It is difficult to understand which roles perform what actions. The different words should be adopted so that an actor is assigned to a single role.
**How to Detect:** –

---

**Name:** Multiple Actors of a Role
**Characteristic:** *Granularity*
**Scope:** *Section*
**Symptom:** The different words are used to represent one actor role. It causes a misunderstanding that these words may denote the different roles of actors. They should be merged into a single word.
**How to Detect:** –

---

**Name:** Long Sentence
**Characteristic:** *Granularity*
**Scope:** *Sentence*
**Symptom:** A sentence is relatively long to the other ones in a section. The target sentence may contain too much information or may contain unnecessary information, which decreases the understandability of the sentence. It should be separated so as to be easier to understand.
**How to Detect:** The number of characters in a sentence (length of a sentence) exceeds a threshold which is calculated by the distribution of the lengths of the sentences among the target use case description? (LOS > $Threshold_{Long}$)

---

**Name:** Short Sentence
**Characteristic:** *Granularity*
**Scope:** *Sentence*
**Symptom:** A sentence is relatively short to the other ones in a section. The target sentence may contain minor information or lack necessary information, which decreases the understandability of the sentence.
**How to Detect:** The number of characters in a sentence (length of a sentence) is less than a threshold which is calculated by the distribution of the lengths of the sentences among the target use case description? (LOS < $Threshold_{Short}$)

---

**Name:** Sentence with Multiple Actions
**Characteristic:** *Granularity*
**Scope:** *Sentence*

**Symptom:** A sentence denotes multiple actions. It should be assigned to a single action.
**How to Detect:** The number of action verbs in a sentence (NOV) exceeds to a threshold? (NOV > 4)

---

**Name:** Relatively Over Qualified Sentence
**Characteristic:** *Granularity*
**Scope:** *Sentence*
**Symptom:** A sentence has relatively many modifiers than other sentences. It may include irrelevant information to understand requirements.
**How to Detect:** The number of modifiers (NOM) exceeds a threshold which is calculated by the distribution of the numbers of the modifiers in sentences among the target use case description? ($\mathsf{NOM} > Threshold_{OverModifier}$)

---

**Name:** Relatively Under Qualified Sentence
**Characteristic:** *Granularity*
**Scope:** *Sentence*
**Symptom:** A sentence has relatively fewer modifiers than other sentences. It may lack relevant information to understand requirements.
**How to Detect:** The number of modifiers (NOM) is less than a threshold which is calculated by the distribution of the numbers of the modifiers in sentences among the target use case description? ($\mathsf{NOM} < Threshold_{UnderModifier}$)

---

**Name:** Omitting Pre-Appeared Word
**Characteristic:** *Granularity*
**Scope:** *Word*
**Symptom:** A word appearing before is omitted in a sentence. Information related to the word may be lacking.
**How to Detect:** –

---

**Name:** Qualified Pre-Appeared Word
**Characteristic:** *Granularity*
**Scope:** *Word*
**Symptom:** A word appearing before is qualified later, i.e., a word is not qualified at the first appearance, but it is qualified in the appearances after the first time. It means that relevant information that the word has was lacking when it appeared for the first time. When it appears at first, it should be qualified.
**How to Detect:** –

---

**Name:** Multiple Flows with the Same Role
**Characteristic:** *Redundancy*
**Scope:** *Flow*
**Symptom:** There are multiple flows whose goals are the same. It may cause the misunderstanding that these multiple flows may have a different meaning.
**How to Detect:** –

---

**Name:** Flow Unrelated to Postcondition
**Characteristic:** *Redundancy*
**Scope:** *Flow*
**Symptom:** Although the postconditions have already held, a flow performs actions not related to the postconditions. These actions may be redundant.
**How to Detect:** –

---

**Name:** Conditional Flow
**Characteristic:** *Redundancy*
**Scope:** *Flow*
**Symptom:** There is a flow where no actions are performed. It may not represent how to use the system to be developed, and can be considered redundant.
**How to Detect:** –

---

**Name:** Repeating the Same Noun
**Characteristic:** *Redundancy*
**Scope:** *Sentence*
**Symptom:** A sentence contains multiple occurrences of the same noun. Although the number of words in the sentence is increasing, there may be no new information obtained from the multiple occurrences of the noun.
**How to Detect:** The number of the occurrences of a noun in a sentence is more than 1? ($\mathsf{NON}(noun) > 1$)

---

**Name:** Over-Qualified Word
**Characteristic:** *Redundancy*
**Scope:** *Word*
**Symptom:** The word *A* together with the modifier *B* appears in the description, but there are no occurrences of the single word *A* or none of the word *A* with the modifier different from *B*. In this case, it may cause the misunderstanding that the word *A* with the different modifier could be missing.
**How to Detect:** –

---

**Name:** Non-Standalone Use Case
**Characteristic:** *Lack*
**Scope:** *Usecase*
**Symptom:** A use case cannot be executed with a standalone. Another use case using it may be lacking.
**How to Detect:** –

---

**Name:** Missing Actor Section
**Characteristic:** *Lack*
**Scope:** *Section*
**Symptom:** There is no actor section in a use case. It is time-consuming to identify actors of the use case.
**How to Detect:** There is no Actor Section in the use case? ($\neg$*ActionSectionExist?*)

---

**Name:** Missing Exception Flows Section
**Characteristic:** *Lack*
**Scope:** *Section*

**Symptom:** There are no exception flow sections in a use case. In this case, we have two alternatives; one is that the use case really has no exception flows, another is that there are no considerations on exception flows yet.

**How to Detect:** There is no exception flows in the use case? (¬*ExceptionFlowSectionExist?*)

---

**Name:** Missing Alternate Flows Section
**Characteristic:** *Lack*
**Scope:** *Section*
**Symptom:** There are no alternate flow sections in a use case. In this case, we have two alternatives; one is that the use case really has no alternate flows, another is that there are no considerations on alternate flows yet.
**How to Detect:** There are no alternate flows in the use case? (¬*AlternateFlowSectionExist?*)

---

**Name:** Missing Preconditions Section
**Characteristic:** *Lack*
**Scope:** *Section*
**Symptom:** There is no section on preconditions. It is not clear when the use case can be executed.
**How to Detect:** There is not a precondition section in the use case? (¬*PreconditionSectionExist?*)

---

**Name:** Missing Postconditions Section
**Characteristic:** *Lack*
**Scope:** *Section*
**Symptom:** There is no section on postconditions. It is not clear what conditions should hold after the use case finishes its execution.
**How to Detect:** There is not a postcondition section in the use case? (¬*PostconditionSectionExist?*)

---

**Name:** Missing Description Section
**Characteristic:** *Lack*
**Scope:** *Section*
**Symptom:** There is no section on describing the overall of a use case. To understand what the use case do roughly, it is time-consuming because we should read all of the use case descriptions.
**How to Detect:** There is not a section on overall description of a use case? (¬*OverviewSectionExist?*)

---

**Name:** Missing Name Section
**Characteristic:** *Section*
**Scope:** *Section*
**Symptom:** There is no section to declare a use case name in a use case description. It is difficult to identify on which use case the descriptions are.
**How to Detect:** There is not a section declaring a use case name? (¬*NameSectionExist?*)

---

**Name:** Premature Exceptional Cases
**Characteristic:** *Lack*
**Scope:** *Flow*
**Symptom:** Every exceptional case that can occur is not described. It is not specified how to deal with the exceptional case that is not described.
**How to Detect:** –

---

**Name:** Premature Branch Condition
**Characteristic:** *Lack*
**Scope:** *Flow*
**Symptom:** Every alternative case that can occur is not described. It is not specified how to deal with the alternative case that is not described.
**How to Detect:** –

---

**Name:** Exception Flow without Return
**Characteristic:** *Lack*
**Scope:** *Sentence*
**Symptom:** There is no information on which sentence the execution returns to when the exception flow finishes, or on what terminate processing should be done after the exception flow. In this case, it is difficult to understand how to finish the use case correctly.
**How to Detect:** The sentence ID to which an exception flow returns is not specified? (¬*ExceptionFlowsReturnExist?*)

---

**Name:** Unexplained Exception Flow
**Characteristic:** *Lack*
**Scope:** *Sentence*
**Symptom:** There is no descriptions on the conditions which an exception can occur. It is difficult to understand why its basic flow is branched to the exception flow.
**How to Detect:** A condition where the exception occurs is not specified in a sentence? (¬*ExceptionFlowsReasonExist?*)

---

**Name:** Alternate Flow without Return
**Characteristic:** *Lack*
**Scope:** *Sentence*
**Symptom:** There is no information on which sentence the execution returns to when the alternate flow finishes, or on what terminate processing should be done after the alternate flow. In this case, it is difficult to understand how to finish the use case correctly.
**How to Detect:** The sentence ID to which an alternate flow returns is not specified? (¬*AlternateFlowsReturnExist?*)

---

**Name:** Unexplained Alternate Flow
**Characteristic:** *Lack*
**Scope:** *Sentence*
**Symptom:** There are no descriptions on the conditions which an alternative can occur. It is difficult to understand why its basic flow is branched to the alternate flow.

**How to Detect:** A condition where the alternative occurs is not specified in a sentence? ($\neg$*ExceptionFlowsReasonExist?*)

---

**Name:** Incomplete System Behavior
**Characteristic:** *Lack*
**Scope:** *Sentence*
**Symptom:** Some of the system behavior to be required is not described. It is impossible to consider the function of the system correctly.
**How to Detect:** –

---

**Name:** Incomplete System Information
**Characteristic:** *Lack*
**Scope:** *Sentence*
**Symptom:** Some information necessary to implement the system is not described. It is difficult to implement the system correctly.
**How to Detect:** –

---

**Name:** Missing Action Target
**Characteristic:** *Lack*
**Scope:** *Word*
**Symptom:** A word that is a target of an action does not appear in a sentence. It is difficult to understand correctly how to use the system.
**How to Detect:** –

---

**Name:** Missing Operation Procedure
**Characteristic:** *Lack*
**Scope:** *Word*
**Symptom:** Some actual operations for the system are not described.
**How to Detect:** –

---

**Name:** Unknown Origin
**Characteristic:** *Lack*
**Scope:** *Word*
**Symptom:** There is no information on the source of newly generated information denoted by a word. It is difficult to check where the information is generated or to validate the correctness of the information.
**How to Detect:** –

---

**Name:** Precondition in Basic Flow
**Characteristic:** *Misplacement*
**Scope:** *Section*
**Symptom:** A precondition is described at the first step of the basic flow.
**How to Detect:** –

---

**Name:** Postcondition in Basic Flow
**Characteristic:** *Misplacement*
**Scope:** *Section*
**Symptom:** A postcondition is described at the last step of the basic flow.
**How to Detect:** –

---

**Name:** Exception Flow in Basic Flow
**Characteristic:** *Misplacement*
**Scope:** *Section*
**Symptom:** An exception flow is described in the basic flow. It is difficult to capture the essential behavior of the use case.
**How to Detect:** –

---

**Name:** Alternate Flow in Basic Flow
**Characteristic:** *Misplacement*
**Scope:** *Section*
**Symptom:** An alternate flow is described in the basic flow. It is difficult to capture the essential behavior of the use case.
**How to Detect:** –

---

**Name:** Synonym
**Characteristic:** *Inconsistency*
**Scope:** *Word*
**Symptom:** The different words having the same meaning is used.
**How to Detect:** –

## References


[1] Y. Seki, S. Hayashi, and M. Saeki, "Detecting bad smells in use case descriptions," to appear in *Proceedings of the 27th IEEE International Requirements Engineering Conference (RE'19)*, 2019.
[2] R. Miles and K. Hamilton, *Learning UML 2.0: A Pragmatic Introduction to UML (Translated in Japanese)*. O'Reilly, 2007.
[3] G. Schneider and J. P. Winters, *Applying Use Cases: A Practical Guide (Translated in Japanese)*. Pearson Education, 2000.
[4] Y. Takaku, S. Hayashi, and M. Saeki, "Generating state transition models from use case descriptions," *IPSJ SIG Technical Reports*, vol. 2010-SE-167, no. 17, pp. 1–8, 2010.
[5] K. T. Phalp, J. Vincent, and K. Cox, "Assessing the quality of use case descriptions," *Software Quality Journal*, vol. 15, no. 1, pp. 69–97, 2007.
[6] F. Tørner, M. Ivarsson, F. Pettersson, and P. Öhman, "Defects in automotive use cases," in *Proceedings of the 5th ACM/IEEE International Symposium on Empirical Software Engineering (ISESE 2006)*, 2006, pp. 115–123.
[7] B. Anda and D. I. K. Sjøberg, "Towards an inspection technique for use case models," in *Proceedings of the 14th International Conference on Software Engineering and Knowledge Engineering (SEKE 2002)*, 2002, pp. 127–134.

TABLE I
USE CASE DESCRIPTIONS USED FOR INSPECTION

| ID | Name | Domain | Description | Source | *B* | *E* | *A* |
|---|---|---|---|---|---|---|---|
| U01 | Move piece on board | Game | Move a piece in hand, take an enemy piece in the target space, or check the enemy king piece to take advantage | https://linuxserver.jp/%E8%A8%AD%E8%A8%88/uml/%E3%83%A6%E3%83%BC%E3%82%B9%E3%82%B1%E3%83%BC%E3%82%B9%E8%A8%98%E8%BF%B0/ ⓢ+ⓤ | 5 | 8 | 2 |
| U02 | Print elterly relief call application form | Welfare | Register the elderly relief telephone application information in the system and output the "Relief telephone application form" | http://archive.city.yokohama.lg.jp/kenko/gohou/jiki-files/c02-sysuc-tb.pdf ⓢ+ⓤ | 9 | 6 | 0 |
| U03 | Display alarm at schedule time | Scheduler | | https://www.ogis-ri.co.jp/otc/hiroba/technical/JavaWorld_UML/chap5/ ⓢ+ⓤ | 4 | 0 | 1 |
| U04 | Process attendance | Business management | Complete the attendance process | http://objectclub.jp/technicaldoc/uml/umlintro2 ⓢ+ⓤ | 6 | 2 | 0 |
| U05 | Operate wiper with washer | Automotive | Wash off oil film, mud, and insects | https://www.zipc.com/event/uc/18th_files2/05-fujiwara.pdf ⓢ+ⓤ | 5 | 0 | 0 |
| U06 | Display | GUI | Display the table created by the actor | https://www.juse.or.jp/sqip/workshop/report/attachs/2008/5-testanalysis-appendix1.pdf ⓢ+ⓤ | 2 | 0 | 0 |
| U07 | Lend works to members | Rental | Lend works to members, collect the lending fee, and record the lending history | https://books.google.co.jp/books?id=rZ3a1beWEUsC&printsec=frontcover ⓢ+ⓤ | 18 | 6 | 5 |
| U08 | Draw shape | GUI | | http://www.fse.cs.ritsumei.ac.jp/lesson/java/practice2.html*2 ⓢ+ⓤ | 5 | 0 | 1 |
| U09 | Load figures from file | GUI | | http://www.fse.cs.ritsumei.ac.jp/lesson/java/practice3.html*2 ⓢ+ⓤ | 6 | 0 | 2 |
| U10 | Get emergency hospitalized | Welfare | | https://www.jahis.jp/...*1 ⓢ+ⓦ | 10 | 0 | 0 |
| U11 | Daily home care | Welfare | | https://www.jahis.jp/...*1 ⓢ+ⓦ | 19 | 0 | 0 |
| U12 | Discharge and transit to home care | Welfare | | https://www.jahis.jp/...*1 ⓢ+ⓦ | 8 | 0 | 0 |
| U13 | Register user | Web | A user who wants to use the bulletin board registers his/her user information in the system | https://www.ibm.com/developerworks/jp/websphere/library/java/web_practice/3.html ⓘ+ⓤ | 13 | 4 | 0 |
| U14 | Register user officially | Web | A temporary user determines his/her official password and logs in to the system | https://www.ibm.com/developerworks/jp/websphere/library/java/web_practice/4.html ⓘ+ⓤ | 9 | 3 | 0 |
| U15 | Initialize password | Web | Re-register as a temporary user when the user has forgotten his/her password | https://www.ibm.com/developerworks/jp/websphere/library/java/web_practice/5.html ⓘ+ⓤ | 8 | 2 | 0 |
| U16 | Log off | Shopping | Discard the order information entered by the customer | https://www.ipa.go.jp/files/000056487.pdf ⓘ+ⓤ | 3 | 0 | 0 |
| U17 | Register order information | Shopping | Receive order details and register order information in the system | https://www.ipa.go.jp/files/000056487.pdf ⓘ+ⓤ | 10 | 0 | 5 |
| U18 | Add item to cart | Shopping | Create a sales order item and calculate the sales order amount with the products and quantities entered by the customer | https://www.ipa.go.jp/files/000056487.pdf ⓘ+ⓤ | 8 | 0 | 3 |
| U19 | Search for product | Shopping | Display the product list by product category | https://www.ipa.go.jp/files/000056487.pdf ⓘ+ⓤ | 4 | 0 | 4 |
| U20 | Log on | Shopping | Authenticate the user and make the system available for him/her | https://www.ipa.go.jp/files/000056487.pdf ⓘ+ⓤ | 3 | 0 | 1 |
| U21 | Register user | Shopping | Entering customer information, the system registers the user with the entered information and issues the user ID | https://www.ipa.go.jp/files/000056487.pdf ⓘ+ⓤ | 8 | 0 | 3 |
| U22 | Create new blog account | Web | A new or existing author requests an administrator for a new blog account | Miles and Hamilton [2] | 6 | 0 | 2 |
| U23 | Place order | Shopping | | Schneider and Winters [3] | 9 | 0 | 1 |
| U24 | Pay consumption tax | Shopping | | Schneider and Winters [3] | 2 | 0 | 0 |
| U25 | Update account | Shopping | Charge or transfer to an account | Schneider and Winters [3] | 4 | 0 | 0 |
| U26 | Send product catalog | Shopping | A customer requests a product catalog | Schneider and Winters [3] | 6 | 0 | 0 |
| U27 | Organize sales report | Shopping | Customer contact gets sales report | Schneider and Winters [3] | 5 | 0 | 0 |
| U28 | Log in | Shopping | | Takaku *et al.* [4] | 2 | 0 | 1 |
| U29 | Log out | Shopping | | Takaku *et al.* [4] | 1 | 0 | 0 |
| U30 | Order | Shopping | | Takaku *et al.* [4] | 2 | 0 | 0 |
| U31 | Lend book | Rental | Receptionist inputs to the system in the lending process | http://msyushi2011.appspot.com/ensyu_sekkei02.jsp ⓢ+ⓤ | 5 | 0 | 2 |
| U32 | Search for product | Shopping | | https://blog.asial.co.jp/831 ⓢ+ⓤ | 3 | 3 | 0 |
| U33 | Register product | Shopping | | https://blog.asial.co.jp/831 ⓢ+ⓤ | 6 | 2 | 0 |
| U34 | Withdraw money with ATM | Finance | Use the bank ATM to withdraw money from the account with a cash card | http://marunomaruno.web.fc2.com/examples/uml/ATMUsecase01.txt ⓢ+ⓤ | 10 | 4 | 6 |
| U35 | Start care service | Welfare | | https://www.jahis.jp/...*1 ⓢ+ⓦ | 12 | 0 | 0 |
| U36 | Register temporal user account | Web | An actor registers user information in the system as a temporary user | https://www.ibm.com/developerworks/jp/websphere/library/java/web_practice/3.html ⓘ+ⓤ | 8 | 2 | 0 |
| U37 | Register user account | Web | A user who wants to use the bulletin board registers his/her user information in the system | https://www.ibm.com/developerworks/jp/websphere/library/java/web_practice/3.html ⓘ+ⓤ | 13 | 3 | 0 |
| U38 | Purchase product | Shopping | | https://qiita.com/putan/items/580cbc6f136859f82edb ⓘ+ⓤ | 5 | 0 | 0 |

ⓢ: Google Search, ⓘ: Google Image Search, ⓤ: Query of "use case description", ⓦ: Query of {"use case description", "welfare"}

*1 https://www.jahis.jp/files/user/04_JAHIS%20standard/14-105_JAHIS%E5%9C%A8%E5%AE%85%E5%8C%BB%E7%99%82%E3%81%A8%E4%BB%8B%E8%AD%B7%E9%96%93%E3%81%AE%E6%83%85%E5%A0%B1%E9%80%A3%E6%90%BA%E3%81%AB%E3%81%8A%E3%81%91%E3%82%8B%E3%83%87%E3%83%BC%E3%82%BF%E9%A0%85%E7%9B%AE%E4%BB%95%E6%A7%98%E6%9B%B8Ver.1.0.pdf

*2 No longer available (accessed: 2019–07–05)

TABLE II
COMPARISON AMONG SMELL CATALOGUES

P: Phalp *et al.* [5]

| | 01 | 02 | 03 | 04 | 05 | 06 | 07 | 08 | 09 | 10 | 11 | 12 | 13 |
|---|---|---|---|---|---|---|---|---|---|---|---|---|---|
| S01: Unordered Flow | | | ✓ | | | | | | ✓ | | | | ✓ |
| S02: Origin-Free Exception Flow | | | | | | | | | | | | | |
| S03: Origin-Free Alternative Flow | | | | | | | | | | | | | |
| S04: Unclear Feasibility | | | | | | | | | | | | | |
| S05: Origin-Free Operation Result | | | | | | | | | | | | | |
| S06: Sentence Interpretable as Multiple Meanings | | | | | | | | | | | | | |
| S07: Pronoun | | | | | | | | | | ✓ | | | |
| S08: Omitted Word | | | | | | | | | | ✓ | | | |
| S09: “Actor” Actor | | | | | | | | | | ✓ | | | |
| S10: Unexplained Main Actor | | | | | | | | | | ✓ | | | |
| S11: Different Concepts by Same Word | | | | | | | | | | ✓ | | | |
| S12: Omitted Attribute | | | | | | | | | | | | | |
| S13: Flow Does Not Meet Precondition | ✓ | | | | ✓ | | | | | | | | |
| S14: Postcondition Not Satisfied | ✓ | | | | ✓ | | | | | | | | |
| S15: Name Does Not Explain Content | ✓ | ✓ | | | ✓ | | | | | | | | |
| S16: Under or Over Condition | ✓ | ✓ | | | ✓ | | | | | | | | |
| S17: Much or Less Actors | ✓ | ✓ | | | | | | | | | | | |
| S18: Contradicted Sentences | | | | | ✓ | | | | | | | | |
| S19: Behavior Ignores Condition | | | | | ✓ | | | | | | | | |
| S20: Multiple Situations | | | | | | | | | | | | | |
| S21: Multiple Exception Flows at an Exception Branch Condition | | | | | | | | | | | | | |
| S22: Multiple Alternate Flows at an Alternate Branch Condition | | | | | | | | | | | | | |
| S23: Multiple Roles of an Actor | | | | | | | | | | | | | |
| S24: Multiple Actors of a Role | | | | | | | | | | | | | |
| S25: Long Sentence | | | | | | | ✓ | | | | | | |
| S26: Short Sentence | | | | | | | ✓ | | | | | | |
| S27: Sentence with Multiple Actions | | | | | | | ✓ | | | | | | |
| S28: Relatively Over Qualified Sentence | | | | | | | ✓ | | | | | | |
| S29: Relatively Under Qualified Sentence | | | | | | | ✓ | | | | | | |
| S30: Omitting Pre-Appeared Word | | | | | | ✓ | | | | | | | |
| S31: Qualified Pre-Appeared Word | | | | | | ✓ | | | | | | | |
| S32: Multiple Flows with the Same Role | | ✓ | | | | | | | | | | | |
| S33: Flow Unrelated to Postcondition | | ✓ | | ✓ | | | | | | | | | |
| S34: Conditional Flow | | | | | | | | | | | | | |
| S35: Repeating the Same Noun | | | | | | | | | | ✓ | | | |
| S36: Over-Qualified Word | | | | | | | | | | | | | |
| S37: Non-Standalone Use Case | | | | | | | | | | | | | |
| S38: Missing Actor Section | | | | | | | | | | | | | |
| S39: Missing Exception Flows Section | | | | | | | | | | | ✓ | | |
| S40: Missing Alternate Flows Section | | | | | | | | | | | ✓ | | |
| S41: Missing Preconditions Section | | | | | | | | | | | | | |
| S42: Missing Postconditions Section | | | | | | | | | | | | | |
| S43: Missing Description Section | | | | | | | | | | | | | |
| S44: Missing Name Section | | | | | | | | | | | | | |
| S45: Premature Exceptional Cases | | | | | | | | | | | ✓ | | |
| S46: Premature Branch Condition | | | | | | | | | | | ✓ | | |
| S47: Exception Flow without Return | | | | | | | | | | | | | |
| S48: Unexplained Exception Flow | | | | | | | | | | | | | |
| S49: Alternative Flow without Return | | | | | | | | | | | | | |
| S50: Unexplained Alternative Flow | | | | | | | | | | | | | |
| S51: Incomplete System Behavior | ✓ | | | | | | | | | | | | |
| S52: Incomplete System Information | ✓ | | | | | | | | | | | | |
| S53: Missing Action Target | ✓ | | | | | | | | | | | | |
| S54: Missing Operation Procedure | ✓ | | | | | | | | | | | | |
| S55: Unknown Origin | ✓ | | | | | | | | | | | | |
| S56: Precondition in Basic Flow | | | | | | | | | | | | | |
| S57: Postcondition in Basic Flow | | | | | | | | | | | | | |
| S58: Exception Flow in Basic Flow | | | | | | | | ✓ | | | | | |
| S59: Alternate Flow in Basic Flow | | | | | | | | ✓ | | | | | |
| S60: Synonym | | | | | | ✓ | | | | | | | |

T: Törner *et al.* [6]

| | 01 | 02 | 03 | 04 | 05 | 06 | 07 | 08 | 09 | 10 | 11 | 12 |
|---|---|---|---|---|---|---|---|---|---|---|---|---|
| S01: Unordered Flow | | | | | ✓ | | | | | | | |
| S02: Origin-Free Exception Flow | | | | | | | | | ✓ | | | |
| S03: Origin-Free Alternative Flow | | | | | | | | | ✓ | | | |
| S04: Unclear Feasibility | | | | | | | | | | | | |
| S05: Origin-Free Operation Result | | | | | | | | | | | | |
| S06: Sentence Interpretable as Multiple Meanings | | | | | | | | | | | | |
| S07: Pronoun | | | | | | | | | | ✓ | | |
| S08: Omitted Word | | | | | | | | | | | | |
| S09: “Actor” Actor | | | | | | | | | | | | |
| S10: Unexplained Main Actor | | | | | | | | | | ✓ | | |
| S11: Different Concepts by Same Word | | | | | | | | | | ✓ | | |
| S12: Omitted Attribute | | | | | | | | | | | | |
| S13: Flow Does Not Meet Precondition | | | | | | | | | | | | ✓ |
| S14: Postcondition Not Satisfied | | ✓ | | | | | | | | | | |
| S15: Name Does Not Explain Content | | | | | | | | | | | | |
| S16: Under or Over Condition | | ✓ | | | | | | | | | | ✓ |
| S17: Much or Less Actors | | | | | | | | | | | | |
| S18: Contradicted Sentences | | | | | | | | | | | | |
| S19: Behavior Ignores Condition | | | | | | | | | | | | ✓ |
| S20: Multiple Situations | | | | | | | | | | | | |
| S21: Multiple Exception Flows at an Exception Branch Condition | | | | | | | | | | | | |
| S22: Multiple Alternate Flows at an Alternate Branch Condition | | | | | | | | | | | | |
| S23: Multiple Roles of an Actor | | | | | | | | | | | | |
| S24: Multiple Actors of a Role | | | | | | | | | | | | |
| S25: Long Sentence | | | | | | ✓ | | | | | ✓ | |
| S26: Short Sentence | | | | | | | | | | | ✓ | |
| S27: Sentence with Multiple Actions | | | | | | ✓ | | | | | ✓ | |
| S28: Relatively Over Qualified Sentence | | | | | | | | | | | ✓ | |
| S29: Relatively Under Qualified Sentence | | | | | | | | | | | ✓ | |
| S30: Omitting Pre-Appeared Word | | | | | | | | | | ✓ | | |
| S31: Qualified Pre-Appeared Word | | | | | | | | | | | | |
| S32: Multiple Flows with the Same Role | | | | | | ✓ | | | | | | |
| S33: Flow Unrelated to Postcondition | | | | ✓ | | ✓ | | | | | | |
| S34: Conditional Flow | | | | | | ✓ | | | | | | |
| S35: Repeating the Same Noun | | | | | | | | | | | ✓ | |
| S36: Over-Qualified Word | | | | | | | | | | ✓ | | |
| S37: Non-Standalone Use Case | | | | | | | | | | | | |
| S38: Missing Actor Section | ✓ | | | | | | | | | | | |
| S39: Missing Exception Flows Section | ✓ | | | | | | | ✓ | | | | |
| S40: Missing Alternate Flows Section | ✓ | | | | | | | ✓ | | | | |
| S41: Missing Preconditions Section | ✓ | | | | | | | | | | | |
| S42: Missing Postconditions Section | ✓ | | | | | | | | | | | |
| S43: Missing Description Section | ✓ | | | | | | | | | | | |
| S44: Missing Name Section | ✓ | | | | | | | | | | | |
| S45: Premature Exceptional Cases | | | | | | | | ✓ | | | | |
| S46: Premature Branch Condition | | | | | | | | ✓ | | | | |
| S47: Exception Flow without Return | | | ✓ | | | | | | | | | |
| S48: Unexplained Exception Flow | | | | | | | | | ✓ | | | |
| S49: Alternative Flow without Return | | | ✓ | | | | | | | | | |
| S50: Unexplained Alternative Flow | | | | | | | | | ✓ | | | |
| S51: Incomplete System Behavior | | ✓ | | | | | | | | | | |
| S52: Incomplete System Information | | ✓ | | | | | | | | | | |
| S53: Missing Action Target | | | | | | | | | | | | |
| S54: Missing Operation Procedure | | | | | | | | | | | | |
| S55: Unknown Origin | | | | | | | | | | | | |
| S56: Precondition in Basic Flow | | | | | | ✓ | | | | | | |
| S57: Postcondition in Basic Flow | | | | | | ✓ | | | | | | |
| S58: Exception Flow in Basic Flow | | | | | | | | ✓ | | | | |
| S59: Alternate Flow in Basic Flow | | | | | | | | ✓ | | | | |
| S60: Synonym | | | | | | | | | | ✓ | | |

A: Anda and Sjøberg [7]

| | 01 | 02 | 03 | 04 | 05 | 06 | 07 | 08 | 09 | 10 | 11 | 12 | 13 | 14 | 15 | 16 | 17 | 18 | 19 | 20 | 21 | 22 | 23 | 24 | 25 | 26 | 27 |
|---|---|---|---|---|---|---|---|---|---|---|---|---|---|---|---|---|---|---|---|---|---|---|---|---|---|---|---|
| S01: Unordered Flow | | | | | | | | | | | | | | | | | | | | | | | | | | | |
| S02: Origin-Free Exception Flow | | | | | | | | | | | | | | | | | | | | | | | | | | | |
| S03: Origin-Free Alternative Flow | | | | | | | | | | | | | | | | | | | | | | | | | | | |
| S04: Unclear Feasibility | | | | | | ✓ | | | | | | | | | | | | | | | | | | | | | |
| S05: Origin-Free Operation Result | | | ✓ | | | ✓ | | | | | | | | | | | | | | | | | | | | | |
| S06: Sentence Interpretable as Multiple Meanings | | | | | | | | | | | | | | | | | | ✓ | | ✓ | ✓ | ✓ | | | | | |
| S07: Pronoun | | | | | | | | | | | | | | | | | | ✓ | | ✓ | ✓ | ✓ | | | | | |
| S08: Omitted Word | | | | | | | | | | | | | | | | | | | | ✓ | ✓ | ✓ | | | | | |
| S09: “Actor” Actor | | | | | | | | | | | | | | | | | | | | | | | | | | | |
| S10: Unexplained Main Actor | ✓ | | | | | | | | | | | ✓ | | | | | | | | | | | | | | | |
| S11: Different Concepts by Same Word | | | | | | | | | | | | | | | | | | | | | | | | | | | |
| S12: Omitted Attribute | | | | | | | | | | | | | | | | | | | | | | | | | | | |
| S13: Flow Does Not Meet Precondition | | | | | | | | | ✓ | ✓ | ✓ | | | | | | | | | | | | | | | | |
| S14: Postcondition Not Satisfied | | | | | | | | | ✓ | ✓ | ✓ | | | | ✓ | | | | | | | | | | | | |
| S15: Name Does Not Explain Content | | | | | | | | ✓ | | | | | | | | | | | ✓ | | | | | | | | |
| S16: Under or Over Condition | | | | | | ✓ | | | | | | | | | | | ✓ | | | | | | | | | | ✓ |
| S17: Much or Less Actors | ✓ | | | | | | | | | | | | | | | | | | | | | | | | | | |
| S18: Contradicted Sentences | | | | | | | | | ✓ | ✓ | | | | | | | | | | | | | | | | | |
| S19: Behavior Ignores Condition | | | | | | | | | ✓ | ✓ | | | | | | | | | | | | | | | | | |
| S20: Multiple Situations | | | | | ✓ | | | | | | | | ✓ | | | | | | | | | | | | | | |
| S21: Multiple Exception Flows at an Exception Branch Condition | | | | | | | | | | | | | | | | | | | | | | | | | | | |
| S22: Multiple Alternate Flows at an Alternate Branch Condition | | | | | | | | | | | | | | | | | | | | | | | | | | | |
| S23: Multiple Roles of an Actor | | | | | | | | | | | | | | | | | | | | | | | | | | | |
| S24: Multiple Actors of a Role | | | | | | | | | | | | | | | | | | | | | | | | | | | |
| S25: Long Sentence | | | | | | | | | | | | | | | | | | | | | | | | | ✓ | | |
| S26: Short Sentence | | | | | | | | | | | | | | | | | | | | ✓ | | | | | | | |
| S27: Sentence with Multiple Actions | | | | | | | | | | | | | | | | | | | | | | | | | ✓ | | |
| S28: Relatively Over Qualified Sentence | | | | | | | | | | | | | | | | | | | | | | | | | ✓ | | |
| S29: Relatively Under Qualified Sentence | | | | | | | | | | | | | | | | | | | | ✓ | | | | | | | |
| S30: Omitting Pre-Appeared Word | | | | | | | | | | | | | | | | | | | | | | | | | | | |
| S31: Qualified Pre-Appeared Word | | | | | | | | | | | | | | | | | | | | | | | | | | | |
| S32: Multiple Flows with the Same Role | | | | | | | | | | | | | | | | | | | | | | | | | | | |
| S33: Flow Unrelated to Postcondition | | | | | | | | | | | | | | ✓ | ✓ | | | | | | | | | | | ✓ | |
| S34: Conditional Flow | | | | | | | | | | | | | | ✓ | | | | | | ✓ | | | | | | | |
| S35: Repeating the Same Noun | | | | | | | | | | | | | | | | | | | | | | | | | | | |
| S36: Over-Qualified Word | | | | | | | | | | | | | | | | | | | | | | | | | | | |
| S37: Non-Standalone Use Case | | | | | | | | | | | | | | | | | | | | | | | | | | | |
| S38: Missing Actor Section | ✓ | | | | | | | | | | | | | | | | | | | | | | | | | | |
| S39: Missing Exception Flows Section | | | | ✓ | | | | | | | | | | | | | | | | | | | | | | | |
| S40: Missing Alternate Flows Section | | | | ✓ | | | | | | | | | | | | | | | | | | | | | | | |
| S41: Missing Preconditions Section | | | | | | ✓ | | | | | | | | | | | | | | | | | | | | | |
| S42: Missing Postconditions Section | | | | | | ✓ | | | | | | | | | | | | | | | | | | | | | |
| S43: Missing Description Section | | ✓ | | | | | | | | | | | | | | | | | | | | | | | | | |
| S44: Missing Name Section | | | | | | | | | | | | | | | | | | | ✓ | | | | | | | | |
| S45: Premature Exceptional Cases | | | | ✓ | | | | | | | | | | | | | | | | | | | | | | | |
| S46: Premature Branch Condition | | | | ✓ | | | | | | | | | | | | | | | | | | | | | | | |
| S47: Exception Flow without Return | | | | | | | | | | | | | | | | | | | | | | | | | | | |
| S48: Unexplained Exception Flow | | | | | | | | | | | | | | | | | | | | | ✓ | | | | | | |
| S49: Alternative Flow without Return | | | | | | | | | | | | | | | | | | | | | | | | | | | |
| S50: Unexplained Alternative Flow | | | | | | | | | | | | | | | | | | | | | ✓ | | | | | | |
| S51: Incomplete System Behavior | | ✓ | | | | | | | | | | | | | | | | | | | | | | | | | |
| S52: Incomplete System Information | | ✓ | | | | | | | | | | | | | | | | | | | | | | | | | |
| S53: Missing Action Target | | | | | | | | | | | | | | | | | | | | | | | | | | | |
| S54: Missing Operation Procedure | | | | | | | | | | | | | | | | | | | | | | | | | | | |
| S55: Unknown Origin | | | | | | | | | | | | | | | | | | | | | | | | | | | |
| S56: Precondition in Basic Flow | | | | | | | | | | | | | | | | | | | | | | | | | | | |
| S57: Postcondition in Basic Flow | | | | | | | | | | | | | | | | | | | | | | | | | | | |
| S58: Exception Flow in Basic Flow | | | | | | | | | | | | | | | | | | | | | | | | | | | |
| S59: Alternate Flow in Basic Flow | | | | | | | | | | | | | | | | | | | | | | | | | | | |
| S60: Synonym | | | | | | | | | | | | | | | | | | | | | | | | | | | |
